# Supplementary material for: Filamentation of Femtosecond Vector Beams
Source: arXiv:2311.00098 ancillary file (2024-12-10)
Supplement: Supplementary file 1 [file SM_Filamentation_VectorBeams.pdf]

**Supplementary Material**

# Filamentation of Femtosecond Vector Beams

Amirreza Sadeghpour[1] and Daryoush Abdollahpour[1,*]

[1]*Department of Physics, Institute for Advanced Studies in Basic Sciences (IASBS), Zanjan 45137-66731, Iran*

(Dated: December 10, 2024)

## I. KERR EFFECT IN AN ISOTROPIC MEDIUM FOR AN ARBITRARY ELLIPTICALLY-POLARIZED INCIDENT FIELD

To explicitly relate the third-order nonlinear optical susceptibility tensor, $\chi^{(3)}$, in isotropic media (such as air) to the Kerr term in the vector-extended version of the standard filamentation model (Eq. (2) in the main text), we start by expressing the third-order nonlinear polarization amplitude at the frequency $(\omega_o + \omega_n + \omega_m)$ as given in [1]

$$\mathcal{P}_i(\omega_o + \omega_n + \omega_m) = \epsilon_0 D \sum_{jkl} \chi^{(3)}_{ijkl}(\omega_0 + \omega_n + \omega_m, \omega_o, \omega_n, \omega_m)\, \mathcal{E}_j(\omega_0)\, \mathcal{E}_k(\omega_n)\, \mathcal{E}_l(\omega_m) \tag{1}$$

where $D$ is the number of distinct permutations of the input frequencies $\omega_o$, $\omega_n$, and $\omega_m$. In this relation, $\mathcal{E}_j$, $\mathcal{E}_k$, and $\mathcal{E}_l$ represent the $j$, $k$, $l$ Cartesian components of the input electric field amplitudes (envelopes) at frequencies $\omega_o$, $\omega_n$, and $\omega_m$, respectively. Here, $\chi^{(3)}_{ijkl}$ denotes the third-order nonlinear optical susceptibility, a fourth-rank tensor. When calculating the nonlinear response at the frequency of the incident field, $\omega$, the input frequencies are $(\omega, \omega, -\omega)$. In this case, the number of distinct permutations of the input frequencies is 3, giving $D = 3$. For simplicity, we adopt the notation $\chi_{ijkl} \equiv \chi^{(3)}_{ijkl}(\omega = \omega + \omega - \omega)$.

For an isotropic medium, such as air, the nonzero elements of the third-order susceptibility tensor are reduced to the following set of equivalent elements, as described in [1]

$$\chi_{1111} = \chi_{2222} = \chi_{3333}, \tag{2a}$$

$$\chi_{1122} = \chi_{1133} = \chi_{2211} = \chi_{2233} = \chi_{3311} = \chi_{3322}, \tag{2b}$$

$$\chi_{1212} = \chi_{1313} = \chi_{2323} = \chi_{2121} = \chi_{3131} = \chi_{3232}, \tag{2c}$$

$$\chi_{1221} = \chi_{1331} = \chi_{2112} = \chi_{2332} = \chi_{3113} = \chi_{3223}. \tag{2d}$$

These equivalences reflect the symmetry properties of the susceptibility tensor in isotropic media. However, the four categories of the nonzero elements in Eqs. (2) are not independent because the nonlinear polarization in isotropic media must be invariant under the rotation of the coordinate system, therefore

$$\chi_{1111} = \chi_{1122} + \chi_{1212} + \chi_{1221}. \tag{3}$$

Using Eqs. (2), and Eq. (3), the compact form the nonlinear susceptibility tensor can be written as

$$\chi_{ijkl} = \chi_{1122}\delta_{ij}\delta_{kl} + \chi_{1212}\delta_{ik}\delta_{jl} + \chi_{1221}\delta_{il}\delta_{jk}. \tag{4}$$

* dabdollahpour@iasbs.ac.ir

Moreover, full permutation symmetry of the nonlinear susceptibility in the case of nonresonant interactions (as in our case) [1] implies that $\chi_{1122} = \chi_{1212} = \chi_{1221}$. Combining this with Eq. (3) we find

$$\chi_{1111} = 3\chi_{1122} = 3\chi_{1212} = 3\chi_{1221}. \tag{5}$$

Thus, the third-order susceptibility at frequency ($\omega = \omega + \omega - \omega$) can be expressed as

$$\chi_{ijkl} = \chi_{1122}(\delta_{ij}\delta_{kl} + \delta_{ik}\delta_{jl} + \delta_{il}\delta_{jk}) = \frac{1}{3}\chi_{1111}(\delta_{ij}\delta_{kl} + \delta_{ik}\delta_{jl} + \delta_{il}\delta_{jk}). \tag{6}$$

For a transverse input electric field (as is the case here, since the diameter of the light filaments exceeds several tens of the wavelength), the nonlinear polarization amplitude along the $i = 1$ axis is expressed as

$$\mathcal{P}_1(\omega) = 3\epsilon_0 \sum_{jkl\in 1,2} \chi_{1jkl}(\omega = \omega + \omega - \omega)\mathcal{E}_j(\omega)\mathcal{E}_k(\omega)\mathcal{E}_l(-\omega). \tag{7}$$

Using Eq.(5), Eq. (6), and noting that $\mathcal{E}(-\omega) = \mathcal{E}^*(\omega)$, Eq. (7) can be expanded to

$$\begin{aligned} \mathcal{P}_1(\omega) &= \epsilon_0\chi_{1111}[|\mathcal{E}_1|^2\mathcal{E}_1 + |\mathcal{E}_2|^2\mathcal{E}_1 + |\mathcal{E}_1|^2\mathcal{E}_1 + |\mathcal{E}_2|^2\mathcal{E}_1 + \mathcal{E}_1^2\mathcal{E}_1^* + \mathcal{E}_2^2\mathcal{E}_1^*] \\ &= \epsilon_0\chi_{1111}[2(\boldsymbol{\mathcal{E}}\cdot\boldsymbol{\mathcal{E}}^*)\mathcal{E}_1 + (\boldsymbol{\mathcal{E}}\cdot\boldsymbol{\mathcal{E}})\mathcal{E}_1^*]. \end{aligned} \tag{8}$$

Similarly, the second component of the nonlinear polarization amplitude can be derived. Thus, the vector form of the nonlinear polarization is given by

$$\boldsymbol{\mathcal{P}}(\omega) = \epsilon_0\chi_{1111}[2(\boldsymbol{\mathcal{E}}\cdot\boldsymbol{\mathcal{E}}^*)\boldsymbol{\mathcal{E}} + (\boldsymbol{\mathcal{E}}\cdot\boldsymbol{\mathcal{E}})\boldsymbol{\mathcal{E}}^*]. \tag{9}$$

This form provides a compact representation of the nonlinear polarization in terms of the electric field components and their interactions. Having established the relationship between the input field envelope and the nonlinear polarization envelope, it is now more convenient to represent both the field and polarization envelopes in the circular polarization basis

$$\boldsymbol{\mathcal{E}} = \mathcal{E}^+\hat{\epsilon}_L + \mathcal{E}^-\hat{\epsilon}_R, \tag{10}$$

$$\boldsymbol{\mathcal{P}} = \mathcal{P}^+\hat{\epsilon}_L + \mathcal{P}^-\hat{\epsilon}_R, \tag{11}$$

where $\hat{\epsilon}_L = \frac{1}{\sqrt{2}}(\hat{\mathbf{x}} + \mathbb{i}\hat{\mathbf{y}})$, and $\hat{\epsilon}_R = \frac{1}{\sqrt{2}}(\hat{\mathbf{x}} - \mathbb{i}\hat{\mathbf{y}})$ are the unit vectors for left-, and right-circular polarizations (LCP, and RCP), respectively. Here, $\mathcal{E}^+$ ($\mathcal{P}^+$), and $\mathcal{E}^-$ ($\mathcal{P}^-$) are the field

(polarization) amplitudes of the LCP and RCP components, respectively. Moreover, it can be easily verified that the LCP and RCP unit vectors have the following properties:

$$\begin{aligned} &\hat{\epsilon}_L^* = \hat{\epsilon}_R, \qquad \hat{\epsilon}_R^* = \hat{\epsilon}_L \\ &\hat{\epsilon}_L \cdot \hat{\epsilon}_L = 0, \quad \hat{\epsilon}_R \cdot \hat{\epsilon}_R = 0, \\ &\hat{\epsilon}_L \cdot \hat{\epsilon}_R = 1, \quad \hat{\epsilon}_R \cdot \hat{\epsilon}_L = 1. \end{aligned} \tag{12}$$

Therefore, the two dot products in the bracket in Eq. (9) can be written as

$$\begin{aligned} \boldsymbol{\mathcal{E}} \cdot \boldsymbol{\mathcal{E}}^* &= |\mathcal{E}^+|^2 + |\mathcal{E}^-|^2, \\ \boldsymbol{\mathcal{E}} \cdot \boldsymbol{\mathcal{E}} &= 2\mathcal{E}^-\mathcal{E}^+. \end{aligned} \tag{13}$$

The nonlinear polarization components along RCP and LCP directions can be calculated by substituting Eq.(13) in Eq. (9), utilizing Eqs. (10)-(11), and applying the orthogonality properties of the unit vectors of circular polarization given in Eqs. (12). For example, the RCP component of the nonlinear polarization envelope ($\mathcal{P}^-$) is calculated as

$$\begin{aligned} \mathcal{P}^- &= \epsilon_0\chi_{1111}[2(\boldsymbol{\mathcal{E}} \cdot \boldsymbol{\mathcal{E}}^*)\mathcal{E}^- + (\boldsymbol{\mathcal{E}} \cdot \boldsymbol{\mathcal{E}})(\mathcal{E}^+)^*] \\ &= \epsilon_0\chi_{1111}[2|\mathcal{E}^-|^2\mathcal{E}^- + 2|\mathcal{E}^+|^2\mathcal{E}^- + 2|\mathcal{E}^+|^2\mathcal{E}^-] \\ &= 2\epsilon_0\chi_{1111}(|\mathcal{E}^-|^2 + 2|\mathcal{E}^+|^2)\mathcal{E}^-. \end{aligned} \tag{14}$$

Similarly, the LCP component of the nonlinear polarization envelope is found as

$$\mathcal{P}^+ = 2\epsilon_0\chi_{1111}(|\mathcal{E}^+|^2 + 2|\mathcal{E}^-|^2)\mathcal{E}^+. \tag{15}$$

These expressions can be compactly written as

$$\mathcal{P}^\pm = 2\epsilon_0\chi_{1111}(|\mathcal{E}^\pm|^2 + 2|\mathcal{E}^\mp|^2)\mathcal{E}^\pm. \tag{16}$$

For a linearly-polarized (LP) input field, $\mathcal{E}$, Eq.(16) is simplified to the familiar form of

$$\mathcal{P}^{\mathrm{LP}} = 3\epsilon_0\chi_{1111}|\mathcal{E}|^2\mathcal{E}, \tag{17}$$

where we have used the fact that $|\mathcal{E}^+|^2 = |\mathcal{E}^-|^2 = \frac{1}{2}|\mathcal{E}|^2$. Equation (17) leads to the well-known relation of the total refractive index in the propagation medium [1]

$$n = n_0 + n_2 I, \tag{18}$$

where $n_0$ represents the linear refractive index, $n_2$ is the Kerr coefficient for the linear polarization, and $I = 2n_0\epsilon_0 c|\mathcal{E}|^2$ denotes the intensity of the incident field (assuming that

there is no linear absorption at the incident frequency). Furthermore, the Kerr coefficient for the linearly polarized field is related to the third-order nonlinear susceptibility as described in [1].

$$n_2 = \frac{3}{4n_0^2\epsilon_0 c}\chi_{1111}. \tag{19}$$

Similarly, the total refractive index for the LCP, and RCP components of an arbitrary elliptically-polarized field in the propagation medium can be written as

$$n^{\pm} = n_0 + n_2'(I^{\pm} + 2I^{\mp}), \tag{20}$$

where $I^{\pm} = 2n_0\epsilon_0 c|\mathcal{E}^{\pm}|^2$, and $n_2'$ is the Kerr coefficient for the elliptically-polarized field. Interestingly, by comparing the nonlinear polarizations given in Eqs. (16) and (17), and the refractive indices given in Eqs. (18) and (20) it is found that

$$n_2' = \frac{2}{3}n_2. \tag{21}$$

Equation (20) can be rewritten using the relation between the Kerr coefficients for the elliptically-, and linearly-polarized fields given in Eq. (21), as

$$n^{\pm} = n_0 + \frac{2}{3}n_2(I^{\pm} + 2I^{\mp}). \tag{22}$$

The second part of Eq. (22) corresponds to the nonlinear refractive index change due to the optical Kerr effect. Notably, as it derived from Eq. (16), it is clearly composed of a self-, and a cross-Kerr contributions. Noting that the field amplitudes in the nonlinear propagation equation (i.e., Eq. (2) of the main text) are defined in such a way that $|\mathcal{E}^{\pm}|^2$ is given in the units of intensity (e.g., W/cm$^2$), the relation for the total refractive index given in Eq. (22) leads to the appearance of the Kerr term in the nonlinear propagation equation as $\mathbb{i}\frac{2}{3}kn_2(|\mathcal{E}^{\pm}|^2 + 2|\mathcal{E}^{\mp}|^2)\mathcal{E}^{\pm}$.

## II. EVOLUTION OF THE FLUENCE AND POLARIZATION PROFILE OF THE CVBs WITH AN INITIAL 10% NOISE

The filamentation of CVBs with an initial uniform amplitude noise, characterized by a correlation length of $0.15w_0$ and a magnitude equal to the 10% of the initial peak amplitude of the fields, is also investigated. All other parameters are identical to those in Section III (A) of the main text. Figure S. 1 illustrates the transverse fluence and polarization profiles of the LCP $LG_{0,1}$ beam and the radial CVB at different propagation distances. The peak intensity and electron density for both beams are presented in Fig. S. 2.

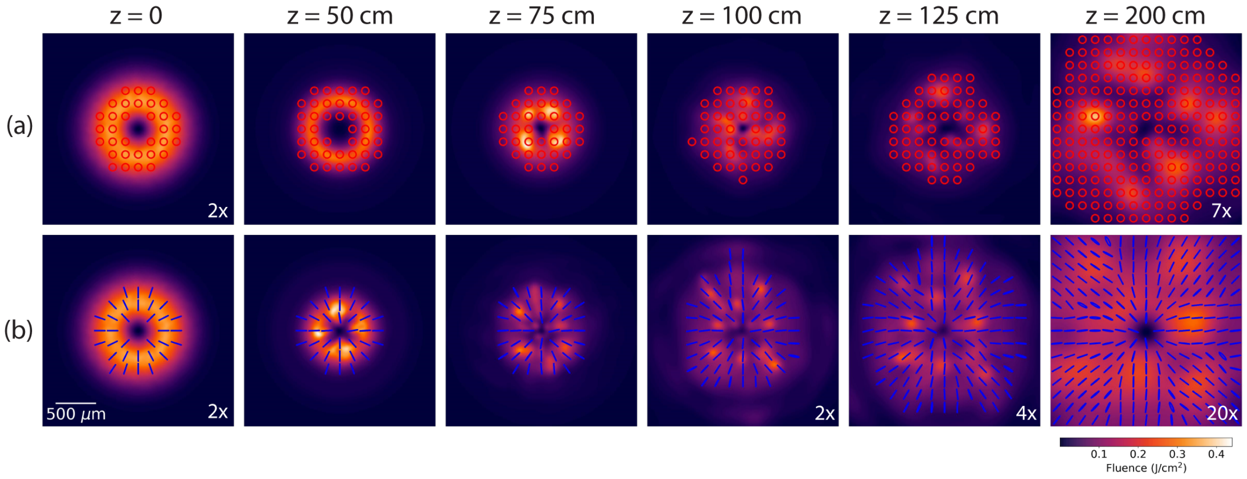


FIG. S. 1. Transverse fluence and polarization profiles of the beams with an initial 10% noise at different propagation distances. (a) LCP $LG_{0,1}$ beam and (b) radial CVBs. In the polarization profiles, red represents left-circular polarization (LCP), while blue indicates linear polarization.

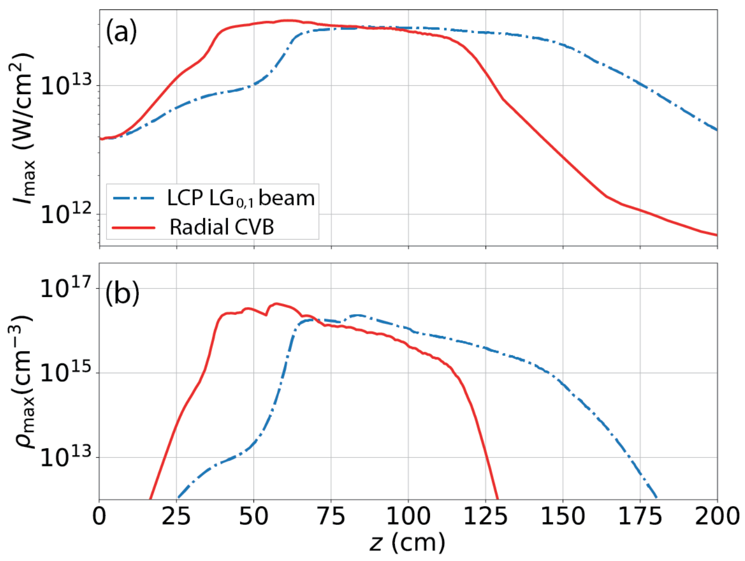


FIG. S. 2. Evolution of maximum intensity (a), and maximum electron density (b) during the filamentation of LCP $LG_{0,1}$ beam and radial CVB, both with an initial 10% noise. Dash-dotted (blue) curve: LCP $LG_{0,1}$ beam; solid (red) curve: radial CVB.

## III. EVOLUTION OF THE FLUENCE AND POLARIZATION PROFILE OF LEMON FPB WITH AN INITIAL 10% NOISE

The filamentation of the lemon FPB and linearly-polarized Gaussian beam, each subjected to uniform amplitude noise with a correlation length of $0.15w_0$ and a magnitude equal to 10% of the initial peak amplitude of the fields, is also examined. All other parameters are identical to those of Section III (B) of the main text. Figure S. 3 illustrates the transverse fluence and polarization profiles of the lemon FPB at various propagation distances. The peak intensity and electron density for both the lemon FPB and the linearly-polarized Gaussian beam are displayed in Fig. S. 4.

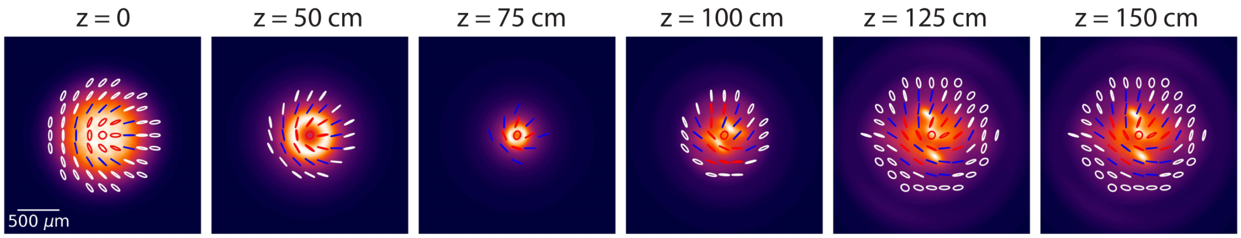


FIG. S. 3. Transverse fluence and polarization profiles of lemon FPB with an initial 10% noise at different propagation distance. In the polarization profiles, red, and white colors represent left-, and right-handed polarization states, respectively; while blue color indicates linear polarization.

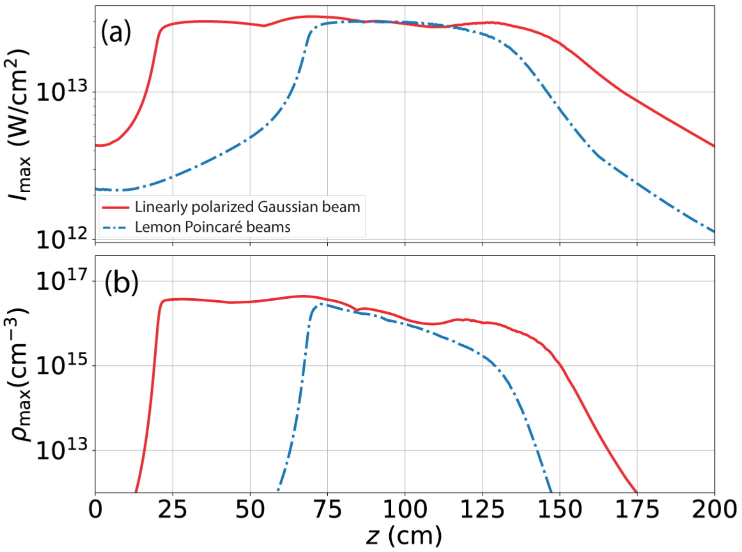


FIG. S. 4. Evolution of maximum intensity (a), and maximum electron density (b) during the filamentation of LP Gaussian beam and the lemon FPB, both with an initial 10% noise. Solid (red) curve: LP Gaussian beam; dash-dotted (blue) curve: lemon FPB.

[1] R. W. Boyd, *Nonlinear Optics*, 4th ed. (Elsevier, 2020).
